# Supplementary material for: Simulating nonlinear dynamics of collective spins via quantum measurement and feedback
Source: arXiv:1907.12606 ancillary file (2020-03-19)
Supplement: Supplementary file 1 [file supplementary_material.pdf]

# Suplementary material for: Simulating nonlinear dynamics of collective spins via quantum measurement and feedback

Manuel H. Muñoz-Arias,[1] Pablo M. Poggi,[1] Poul S. Jessen,[2] and Ivan H. Deutsch[1]

[1] *Center for Quantum Information and Control, CQuIC, Department of Physics and Astronomy, University of New Mexico, Albuquerque, New Mexico 87131, USA*

[2] *Center for Quantum Information and Control, CQuIC, College of Optical Sciences and Department of Physics, University of Arizona, Tucson, AZ 85721, USA*

## CONTENTS

I. Derivation of the average map 1
A. The dephasing rate $\Gamma$ 2

II. The co-moving Holstein-Primakoff approximation and calculation of $\Lambda_{\text{Largest}}$ 2
A. Probability distribution of $m$ 3
B. Co-moving H-P approximation 4
1. Validity of the Holstein-Primakoff approximation 5
C. Explicit form of the map 5
1. On the optimal value of $\sigma$ for the conditioned evolution 6
D. Calculation of $\Lambda_{\text{Largest}}$ 7
E. Convergence of $\Lambda_{\text{Largest}}$ towards the classical value, the quantum to classical transition in the chaotic regime 7

III. The atom-light interface, optical pumping and stochastic master equation 8

References 10

## I. DERIVATION OF THE AVERAGE MAP

In this supplement we derive the evolution of the mixed state, Eq. (5) in the main text, obtained as a weighted average over all possible measurement outcomes

$$\rho_{i+1} = \sum_m P_m \rho_i^{(m)} = \sum_m \hat{K}^{(m)}_{\text{map}} \rho_i \hat{K}^{(m)\dagger}_{\text{map}}, \tag{1}$$

where $\rho_i^{(m)} = \frac{\hat{K}^{(m)}_{\text{map}} \rho_i \hat{K}^{(m)\dagger}_{\text{map}}}{P_m}$, $\hat{K}^{(m)}_{\text{map}} = e^{ip\hat{J}_y} e^{i\frac{k}{J} m \hat{J}_m} \hat{K}_m$. Here we have fixed the feedback policy to be the one giving the KT dynamics, and the Kraus operator $\hat{K}_m$ is defined in Eq. (1) in the main text. Given that the measurement outcome comes from reading the meter, in principle the range of values for $m$ is continuous. The sum in Eq. (1) can then be replaced by an integral,

$$\rho_{i+1} = e^{ip\hat{J}_y} \mathcal{I}(k) e^{-ip\hat{J}_y} = \frac{1}{\sqrt{2\pi\sigma^2}} e^{ip\hat{J}_y} \left[ \int_{-\infty}^{\infty} dm\, e^{i\frac{k}{J} m \hat{J}_z} e^{\frac{1}{4\sigma^2}(\hat{J}_z - m)^2} \rho_i e^{\frac{1}{4\sigma^2}(\hat{J}_z - m)^2} e^{-i\frac{k}{J} m \hat{J}_z} \right] e^{-ip\hat{J}_y}, \tag{2}$$

where $\mathcal{I}(k)$ is an operator valued integral defined by the expression within square brackets in the right hand side of Eq. (2).

To compute the integral we keep track of those operators acting on the state from the right and the ones doing it from the left. In other words, we define left and right acting superoperators as $\hat{J}_z^{\text{L}} \rho_i = \hat{J}_z \rho_i$ and $\hat{J}_z^{\text{R}} \rho_i = \rho_i \hat{J}_z$ [1]. With this definition we can rewrite the integral as a superoperator map

$$\mathcal{I}(k) = \frac{1}{\sqrt{2\pi\sigma^2}} \int_{-\infty}^{\infty} dm\, e^{-i\frac{km}{J}\left(\hat{J}_z^{\text{L}} - \hat{J}_z^{\text{R}}\right)} e^{-\frac{1}{4\sigma^2}\left(\left(\hat{J}_z^{\text{L}} - m\right)^2 + \left(\hat{J}_z^{\text{R}} - m\right)^2\right)} \rho_i, \tag{3}$$

which is a Gaussian integral in the measurement outcome $m$. In order to see this, we expand the powers and reorganize terms to arrive at the expression

$$\mathcal{I}(k) = \frac{e^{-\frac{1}{4\sigma^2}}}{\sqrt{2\pi\sigma^2}} \int_{-\infty}^{\infty} dm\, e^{-\frac{1}{2\sigma^2}\left(m^2 - \left[\hat{J}_z^{\rm L} + \hat{J}_z^{R} + i\frac{2\sigma^2 k}{J}\left(\hat{J}_z^{\rm L} - \hat{J}_z^{\rm R}\right)\right] m\right)} \rho_i. \tag{4}$$

After completing the square and computing the Gaussian integral, we arrive at

$$\mathcal{I}(k) = e^{i\frac{k}{2J}\left(\hat{J}_z^{\rm L2} - \hat{J}_z^{\rm R2}\right)} e^{-\left(\frac{1}{8\sigma^2} + \frac{\sigma^2 k^2}{2J^2}\right)\left(\hat{J}_z^{\rm L} - \hat{J}_z^{\rm R}\right)^2} \rho_i. \tag{5}$$

In order to write the final expression for the stroboscopic map evolving $\rho_i$, we remove the "left" and "right" labels from our operators. To do this we reëxpresse the two exponentials in Eq. (5). First, we consider

$$e^{-\Gamma\left(\hat{J}_z^{\rm L} - \hat{J}_z^{\rm R}\right)^2} \rho = \sum_{s=0}^{\infty} \frac{(-\Gamma)^2}{s!} \left(\left(\hat{J}_z^{\rm L} - \hat{J}_z^{\rm R}\right)^2\right)^s \rho = \sum_{s=0}^{\infty} \frac{\left[-\Gamma \hat{J}_z, \left[\hat{J}_z, \rho\right]\right]^2}{s!} \rho = e^{\Gamma \mathcal{L}_D} \rho, \tag{6}$$

for any density operator $\rho$, where $\Gamma = \frac{1}{8\sigma^2} + \frac{\sigma^2 k^2}{2J^2}$ is the dephasing strength and $\mathcal{L}_D[\rho] = -\left[\hat{J}_z, \left[\hat{J}_z, \rho\right]\right]$. Similarly, the second exponential reads

$$e^{i\frac{k}{2J}\left(\hat{J}_z^{\rm L2} - \hat{J}_z^{\rm R2}\right)} \rho = \sum_{s=0}^{\infty} \frac{\left(\frac{ik}{2J}\right)^s}{s!} \left(\hat{J}_z^{\rm L2} - \hat{J}_z^{\rm R2}\right)^s \rho = \sum_{s=0}^{\infty} \frac{1}{s!} \left[\frac{ik}{2J} \hat{J}_z^2, \rho\right]^s = e^{i\frac{k}{2J}\hat{J}_z^2} \rho\, e^{-i\frac{k}{2J}\hat{J}_z^2}. \tag{7}$$

where the last equality follows from Baker-Campbell-Haussdorf. Putting together the results in Eq. (6), Eq. (7) and Eq. (3) we get the final expression for the stroboscopic map evolving $\rho_i$

$$\rho_{i+1} = e^{ip\hat{J}_y} e^{i\frac{k}{2J}\hat{J}_z^2} e^{\mathcal{L}_D}[\rho_i] e^{-i\frac{k}{2J}\hat{J}_z^2} e^{-ip\hat{J}_y} = \hat{U}_{\rm QKT}\, e^{\mathcal{L}_D}[\rho_i] \hat{U}_{\rm QKT}^{\dagger}, \tag{8}$$

corresponding to a dephased version of the QKT dynamics, where the Floquet operator of the QKT is given by $\hat{U}_{\rm QKT} = e^{ip\hat{J}_y} e^{i\frac{k}{2J}\hat{J}_z^2}$.

### A. The dephasing rate $\Gamma$

In the previous section we showed how one can, for the feedback policy $f(m) = m$ compute analytically the form of the average map. This averaged evolution consists of the unitary operator of the quantum kicked top plus dephasing. One can then ask how long one can access the unitary dynamics before the dephasing washes out signatures of coherent dynamics. In order to analyze this, we need first to fix a value of the measurement strength $\sigma$. Notice that $\Gamma$ is a sum of a term coming from the measurement backaction and a term coming from the feedback, and as such it must have a minimum. To find this minimum, let us write $\sigma = \alpha\sqrt{J}$, where $\alpha$ is a proportionality factor. Then we can write a dephasing strength independent of the size of the spin as

$$\tilde{\Gamma} = \frac{k^2\alpha^2}{2} + \frac{1}{8\alpha^2}, \tag{9}$$

where we ahve defined $\tilde{\Gamma} = \Gamma J$. It thus follows that the optimal value of the measurement strength is determined by

$$\alpha_{opt} = \frac{1}{\sqrt{2k}}, \tag{10}$$

corresponding to a minimum of the dephasing strength of $\tilde{\Gamma} = \frac{k}{2}$. A similar analysis can be done in the case of the stochastic map giving the evolution over an individual trajectory, as we present on Sect. III C.

## II. THE CO-MOVING HOLSTEIN-PRIMAKOFF APPROXIMATION AND CALCULATION OF $\Lambda_{\rm Largest}$

In this supplement we show how to simulate the time evolution of the state $|\psi\rangle_i \to |\psi\rangle_{i+1}$ under the proposed map when one uses the co-moving Holstein-Primakof (H-P) approximation [2]. For weak squeezing introduced by the measurement we can use the Gaussian approximation to obtain an efficient representation of the map. Using the H-P representation, we describe the collective spin operators as corresponding to a bosonic mode, whose phase space corresponds to a tangent plane on the sphere. Once in the plane, we explicitly write the Kraus operator and compute its action on the state. After the state is updated by the measurement, we go back to the original basis (fixed Cartesian basis) and apply the unitary part of the map, which correspond to a pair of rotations.

### A. Probability distribution of $m$

The first step in the conditioned evolution (quantum trajectory) is to perform a sampling procedure to obtain a measurement outcome. In the Gaussian approximation, the form of the distribution can be explicitly computed. Recall that, at step $i$ the distribution is given by

$$P_m = {}_i\langle\psi|\hat{K}_m^\dagger \hat{K}_m|\psi\rangle_i. \tag{11}$$

Since the state remains Gaussian under the action of this map, it can be expressed (in the basis of $\hat{J}_z$) as

$$|\psi\rangle_i = \sum_{M_z=-J}^{J} \frac{1}{\left(2\pi\Delta J_{z,i}^2\right)^{1/4}} e^{-\frac{(M_z-\langle\hat{J}_z\rangle_i)^2}{4\Delta J_{z,i}^2}} |J, M_z\rangle, \tag{12}$$

where $\Delta J_{z,i}^2$ is the spin projection noise of the current state $|\psi\rangle_i$. Since we are implementing an unsharp measurement of $\hat{J}_z$ the Kraus operator is diagonal in this basis, it reads

$$\hat{K}_m = \sum_{M_z=-J}^{J} \frac{1}{\left(2\pi\sigma^2\right)^{1/4}} e^{-\frac{1}{4\sigma^2}(M_z-m)^2} |J, M_z\rangle\langle J, M_z|. \tag{13}$$

Replacing Eq. (12) and Eq. (13) into Eq. (11) we get

$$P_m = \frac{1}{\sqrt{2\pi\Delta J_{z,i}^2}} \frac{1}{\sqrt{2\pi\sigma^2}} e^{-\frac{\langle\hat{J}_z\rangle^2}{2\Delta J_{z,i}^2}} e^{-\frac{m^2}{2\sigma^2}} e^{\frac{\Delta J_{z,i}^2 m_n^2}{2}} \int dM_z e^{-\frac{1}{2\sigma_n^2}\left(M_z-\sigma_n^2 m_n\right)^2}, \tag{14}$$

where using the Gaussian approximation ($J \gg 1$) we replace the summation by an integral $\sum_{M_z} \to \int dM_z$. Furthermore, note that $\sigma_n^2 = \frac{\Delta J_{z,i}^2\sigma^2}{\Delta J_{z,i}^2+\sigma^2}$, and $m_n^2 = \frac{\sigma^4\langle\hat{J}_z\rangle_i^2+\Delta J_{z,i}^4 m^2+2\sigma^2\Delta J_{z,i}^2\langle\hat{J}_z\rangle_i m}{\Delta J_{z,i}^4\sigma^4}$. The integral in Eq. (14) is Gaussian in $M_z$, so we can compute it exactly. After doing so and rearranging terms one finds the following expression for the distribution $P_m$,

$$P_m = \frac{1}{\sqrt{2\pi\left(\Delta J_{z,i}^2+\sigma^2\right)}} e^{-\frac{1}{2\left(\Delta J_{z,i}^2+\sigma^2\right)}\left(m-\langle\hat{J}_z\rangle_i\right)^2}. \tag{15}$$

This distribution is a Gaussian centered at the expected value of $\hat{J}_z$ and with a width that changes from evolution step to evolution step.

In the proposed experimental framework for implementing this protocol using the atom-light interface discussed in the main text, the sampling of a measurement outcome is carried out as follows. In the polarization spectroscopy experiment the measurement outcome is obtained as the average of the continuous signal $\mathcal{M}(t)$ up to the time $T$ representing the time window during which the measurement is taking place. This approach to obtain the measurement outcome $m$ is statistically equivalent to that obtained from the Kraus operator. To see this, divide the time interval $T$ into $p$ small time bins $\delta t = \frac{T}{p}$ and consider a Kraus operator for each time bin of the form

$$\hat{K}_{m_i} \propto e^{-\frac{(\hat{J}_z-m_i)^2}{4\sigma_{T/p}^2}}, \text{ with } \sigma_{T/p}^2 = \frac{1}{\kappa\delta t} = \frac{p}{\kappa T} = p\sigma^2, \tag{16}$$

where $m_i$ is the measurement outcome for the $i^{th}$ time bin. Now, the continuous signal $\mathcal{M}(t)$ can be constructed as a product of these Kraus operators. And the product covering the $p$ time bins in the time interval $T$ is given by

$$\hat{K}_{m_p}(T/p)\hat{K}_{m_{p-1}}(T/p)...\hat{K}_{m_2}(T/p)\hat{K}_{m_1}(T/p) \propto e^{-\frac{1}{4\sigma^2}\left(\hat{J}_z-\overline{m}\right)^2} \prod_{\substack{i,j=1\\ i\neq j}}^{p} e^{-\frac{1}{p^2 4\sigma^2}(m_i-m_j)^2}, \tag{17}$$

where $\overline{m} = \frac{1}{p}\sum_{i=1}^{p} m_i$ the discretized version of the average of the continuous signal $\mathcal{M}(t)$. Two remarks are necessary here. First, there are $C_2^p = \binom{p}{2}$ terms in the product on the right hand side of Eq. (17). Second, in the limit $p \gg 1$ or $\delta t \to 0$, as is the case in a continuous measurement [3], the product in th right hand side or Eq. (17) goes to 1 and the product of Kraus operators covering the timeinterval $T$ converges to the single one used in our map. In this case, one can use the steps presented from Eq. (11) to Eq. (15) to show that the distribution from which $\overline{m}$ is sampled is the same as that in Eq. (15).

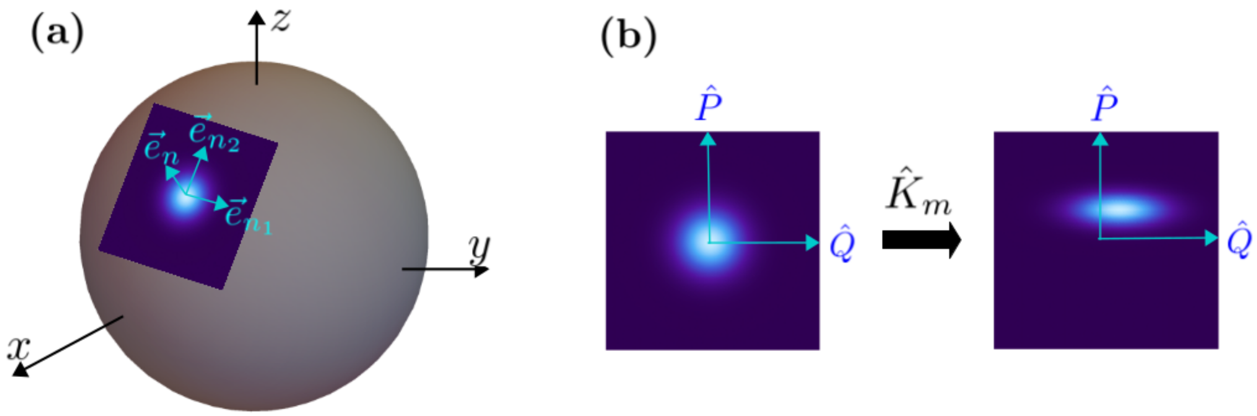


Figure 1. **(a)** Representation of the Gaussian state in the H-P plane, and our choice of local basis. **(b)** Once in the H-P plane, consequences of the action of $\hat{K}_m$ on the state. Random kick and squeezing along the $\hat{P}$ quadrature on the plane.

### B. Co-moving H-P approximation

Under the Gaussian approximation, we can fully represent the state using nine real numbers: the vector of mean values and the covariance matrix, defined by

$$\boldsymbol{n} = \frac{\langle \hat{\boldsymbol{J}} \rangle}{J}, \text{ and } \mathbb{V}_{\alpha,\beta} = \frac{1}{2J}\left( \langle \{ \hat{J}_\alpha, \hat{J}_\beta \} \rangle - 2\langle \hat{J}_\alpha \rangle \langle \hat{J}_\beta \rangle \right), \tag{18}$$

where $\alpha, \beta = x, y, z$, and $\boldsymbol{n}, \mathbb{V}$ correspond to the normalized vector of expectation values and covariance matrix, respectively. Given the vector $\boldsymbol{n}$, we define the perpendicular direction to the H-P plane on the sphere as

$$\vec{e}_{\boldsymbol{n}} \leftrightarrow (\theta, \phi), \text{ with } \theta = \cos^{-1}(\boldsymbol{n}_z), \text{ and } \phi = \tan^{-1}\left( \frac{\boldsymbol{n}_y}{\boldsymbol{n}_x} \right). \tag{19}$$

Recall that the only states which lie on the surface of the sphere, i.e. with $|\boldsymbol{n}| = 1$ are spin coherent states (SCSs), and that any other Gaussian state will have $|\boldsymbol{n}| < 1$. Once we fix the perpendicular direction, we fix the two directions on the H-P plane as follows. We choose $\boldsymbol{e}_{\boldsymbol{n_2}}$, in the direction of $\boldsymbol{e}_z \times \boldsymbol{e}_n$ and remaining direction is chosen according to $\boldsymbol{e}_{\boldsymbol{n_1}} = \boldsymbol{e}_{\boldsymbol{n_2}} \times \boldsymbol{e}_{\boldsymbol{n}}$ (see Fig. 1a).

A change of basis to the local basis on the plane is achieved by a rotation matrix $\mathbb{A}$, given by

$$\mathbb{A} = \begin{pmatrix} -\sin(\phi) & \cos(\phi) & 0 \\ -\cos(\theta)\cos(\phi) & -\cos(\theta)\sin(\phi) & \sin(\theta) \\ \sin(\theta)\cos(\phi) & \sin(\theta)\sin(\phi) & \cos(\theta) \end{pmatrix} \tag{20}$$

which transforms the vector of expected values and covariance matrix in Eq. (18) as

$$\boldsymbol{n}' = \mathbb{A}\boldsymbol{n}, \text{ and } \mathbb{V}' = \mathbb{A}\mathbb{V}\mathbb{A}^T. \tag{21}$$

In the H-P approximation, we have a simple representation of the collective spin operators. First we use $\mathbb{A}$ to change components to the local H-P plane, $\left(\hat{J}_x, \hat{J}_y, \hat{J}_z\right) \to \left(\hat{J}_{n_1}, \hat{J}_{n_2}, \hat{J}_n\right)$. Under the H-P approximation, the operator along the direction normal to the plane is replaced by the classical magnitude and the other two components are mapped to bosonic quadrature operators,

$$\hat{J}_n \to J, \quad \hat{J}_{n_1} \to \sqrt{J}\hat{Q}, \text{ and } \hat{J}_{n_2} \to \sqrt{J}\hat{P}. \tag{22}$$

In the local basis the Kraus operator for unsharp measurement, then takes the form

$$\hat{K}_m \propto e^{-\frac{J\sin^2\theta}{4\sigma^2}\hat{P}^2} e^{\frac{\sqrt{J}\sin\theta m_\theta}{2\sigma^2}\hat{P}}, \tag{23}$$

where we have used $\hat{J}_z - m = \sqrt{J}\hat{P}\sin\theta - m_\theta$, with $m_\theta = m - J\cos\theta$; we do not include the normalization factor. The action of this Kraus operator over the state is twofold. In Eq. (23) the first exponential introduces squeezing of

the bosonic mode with resolution $\sigma/(\sqrt{J}\sin\theta)$ and the second one gives a random kick along the $z$ axis depending on the measurement outcome (see Fig. 1b for an illustration of this effect).

In order to get an expression for the updated version of the state after the measurement, we apply $\hat{K}_m$ as in Eq. (23), now represented as a Gaussian distribution with respect to the bosonic quadratures $(\hat{Q}, \hat{P})$. The measurement only updates the components of $\boldsymbol{r}'$ and $\mathbb{V}'$ corresponding to the two directions on the plane. The vector of expectation values is updated as

$$\boldsymbol{n}'_{n_1} \to \boldsymbol{n}'_{n_1} + \mathbb{V}'_{n_1,n_2}\frac{\sin(\theta)}{\sigma^2}m_\theta, \text{ and } \boldsymbol{n}'_{n_2} \to \boldsymbol{n}'_{n_2} + \mathbb{V}'_{n_2,n_2}\frac{\sin(\theta)}{\sigma^2}m_\theta. \tag{24}$$

The respective subblock of the covariance matrix is updated as

$$\mathbb{V}'_{n_2,n_2} \to \mathbb{V}'_{n_2,n_2}\frac{s^2}{2\mathbb{V}'_{n_2,n_2}+s^2}, \tag{25a}$$

$$\mathbb{V}'_{n_1,n_2} \to \mathbb{V}'_{n_1,n_2}\frac{s^2}{2\mathbb{V}'_{n_2,n_2}+s^2}, \tag{25b}$$

$$\mathbb{V}'_{n_1,n_1} \to \mathbb{V}'_{n_1,n_1} + \frac{1}{2}\left(\frac{1}{s^2} - \frac{4\mathbb{V}'^2_{n_1,n_2}}{2\mathbb{V}'_{n_2,n_2}+s^2}\right), \tag{25c}$$

where $s^2 = \frac{2\sigma^2}{J\sin(\theta)}$. Finally, we transform back to the original basis by rotating with $\mathbb{A}^T$. Once in the fixed Cartesian frame, the unitary part of the map acts trivially by rotating $\boldsymbol{r}$ and $\mathbb{V}^{(r)}$. With this, a single evolution step of our map in the H-P approximation is completed.

### 1. *Validity of the Holstein-Primakoff approximation*

To understand validity of the H-P approximation, note that here one represents the state of a collective spin system by the vacuum state of a bosonic mode whose origin in phase space is a co-moving frame. Whereas the collective spin has the geometry of SO(3) and thus it can be identified with a sphere, the bosonic mode "lives" on a plane. In the H-P approximation one is fundamentally neglecting the curvature of the state space of the spin system. Under our protocol there are two main routes along which the approximation might fail. First, consider a scenario in which the amount of squeezing introduced as a consequence of measurement backaction is too large. In this case the direction being anti-squeezed develops a large support on the sphere and the arc it describes is not longer well approximated by a straight line on a plane. In our protocol, however, this is not the case because we working at the optimal measurement strength $\sigma \sim 1$. That is, the time over which the measurement takes place is far from the time over which significant spin squeezing occurs [4, 5]. Furthermore, as the evolution proceeds and the unitary part of the map rotates the state to a different position on the sphere, the quadratures that are squeezed and anti-squeezed change from one evolution step to the next, yielding an almost vanishing overall squeezing of the state.

The second possible failure mechanism occurs for small ensembles of spins. As discussed above, we can well approximate the state at all times as a spin coherent state, with negligible squeezing. As the uncertainty path for $N$ spin is of order $\sqrt{N}$ and the radius of the collective spin sphere is of order $N$ as long as $N \gg \sqrt{N}$ the uncertainty patch is a negligible fraction of the sphere, and we expect the H-P approximation to be good. This implies $N \gg 100$, which is consistent with the ensemble sizes for the cases we consider in this work.

## C. Explicit form of the map

We can use the H-P approximation to write a Floquet map of the mean values and the covariance matrix that describe the Gaussian state. To do this, first recall that the unitary part of the map acts on the Gaussian state as a pair of rotation matrices,

$$\mathcal{R}_y(-p) = \begin{pmatrix} \cos(p) & 0 & -\sin(p) \\ 0 & 1 & 0 \\ \sin(p) & 0 & \cos(p) \end{pmatrix}, \text{ and } \mathcal{R}_z\left(-\frac{km}{J}\right) = \begin{pmatrix} \cos(\beta_m) & \sin(\beta_m) & 0 \\ -\sin(\beta_m) & \cos(\beta_m) & 0 \\ 0 & 0 & 1 \end{pmatrix}, \tag{26}$$

which correspond to the free rotation around the $y$-axis and the conditioned rotation around the $z$-axis, respectively, with $\beta_m = \frac{km}{J}$. Furthermore let us denote $\boldsymbol{n}''$ and $\mathbb{V}''$ as the vector of mean values and covariance matrix after the

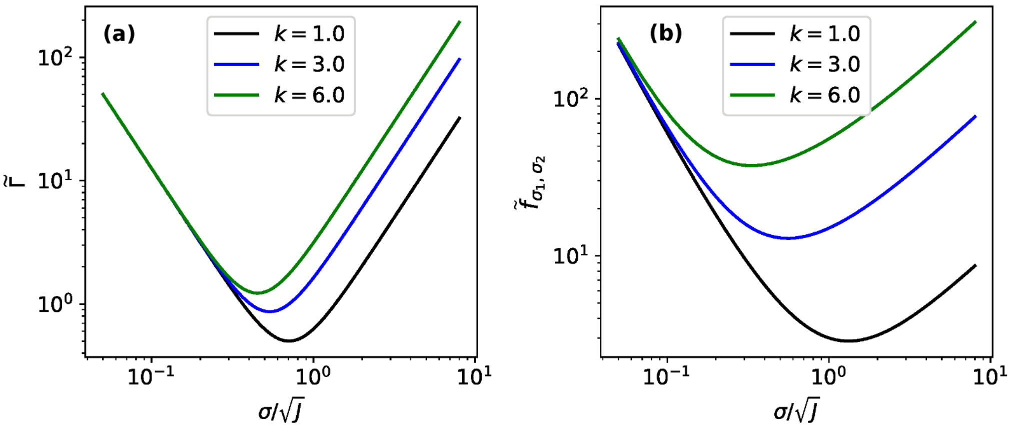


Figure 2. **(a)** Example curves of $\tilde{\Gamma}$ in Eq. (9) as a function of $\alpha = \sigma/\sqrt{J}$. Notice the clear existence of a minimum, signaling the optimal value of $\alpha$. **(b)** Example curves of $\tilde{f}_{\sigma_1,\sigma_2}$ in Eq. (31). Here the existence of a minimum for the convex combination $\sigma_1^2 + \sigma_2^2$ is made evident.

action of the measurement, with the components expressed in the original fixed Cartesian basis. Then, these two objects are evolved under the two rotations as

$$\boldsymbol{n}_{i+1} = \mathcal{R}_y(-p)\mathcal{R}_z(-\beta_m)\boldsymbol{n}'', \tag{27a}$$

$$\mathbb{V}_{i+1} = \mathcal{R}_y(-p)\mathcal{R}_z(-\beta_m)\mathbb{V}''\mathcal{R}_z^T(-\beta_b)\mathcal{R}_y^T(-p). \tag{27b}$$

Introducing the explicit form of the rotations in Eq. (26) into Eq. (27a) and defining $(X, Y, Z) = \boldsymbol{n}$, we find that one evolution step of this vector can be cast in the form of the following stroboscopic map,

$$X_{i+1} = -Z_i - \frac{m_\theta}{\sigma^2}\mathbb{V}_{22}\left(1 - Z_i^2\right), \tag{28a}$$

$$Y_{i+1} = \left(1 - \frac{m_\theta \mathbb{V}_{22}}{\sigma^2}\right)\left(Y_i\cos(\beta_m) - X_i\sin(\beta_m)\right) + \frac{m_\theta \mathbb{V}_{12}}{\sigma^2}\left(X_i\cos(\beta_m) + Y_i\sin(\beta_m)\right), \tag{28b}$$

$$Z_{i+1} = \left(1 - \frac{m_\theta \mathbb{V}_{22}}{\sigma^2}Z_i\right)\left(X_i\cos(\beta_m) + Y_i\sin(\beta_m)\right) - \frac{m_\theta \mathbb{V}_{12}}{\sigma^2}\left(Y_i\cos(\beta_m) - X_i\sin(\beta_m)\right). \tag{28c}$$

From the form of the distribution, in Eq. (15), it follows that $m$ is a Gaussian random variable with mean $\langle \hat{J}_z\rangle_i = J\cos(\theta)$ and variance $\sigma^2 + \Delta J_{z,i}^2$. Thus, we can write

$$\frac{m_\theta}{\sigma^2} \equiv \eta_1 \approx \mathcal{N}(0, \sigma_1^2), \quad \text{with} \quad \sigma_1^2 = \frac{\sigma^2 + \Delta J_{z,i}^2}{\sigma^4}, \tag{29a}$$

$$\frac{m_\theta}{J/k} \equiv \eta_2 \approx \mathcal{N}(0, \sigma_2^2), \quad \text{with} \quad \sigma_2^2 = k^2\frac{\sigma^2 + \Delta J_{z,i}^2}{J^2}. \tag{29b}$$

In terms of these two new random variables the stroboscopic map for the Cartesian components of the normalized vector of expected values takes the form

$$X_{i+1} = -Z_i + \eta_1\mathbb{V}_{22}\left(1 - Z_i^2\right), \tag{30a}$$

$$Y_{i+1} = \left(1 - \eta_1\mathbb{V}_{22}Z_i\right)\left(Y_i\cos\left(kZ_i + \eta_2\right) - X_i\sin\left(kZ_i + \eta_2\right)\right) + \eta_1\mathbb{V}_{12}\left(X_i\cos(kZ_i + \eta_2) + Y_i\sin(kZ_i + \eta_2)\right), \tag{30b}$$

$$Z_{i+1} = \left(1 - \eta_1\mathbb{V}_{22}Z_i\right)\left(Y_i\cos(kZ_i + \eta_2) + Y_i\sin(kZ_i + \eta_2)\right) - \eta_1\mathbb{V}_{12}(Y_i\cos(kZ_i + \eta_2) - X_i\sin(kZ_i + \eta_2)). \tag{30c}$$

### *1. On the optimal value of $\sigma$ for the conditioned evolution*

As presented in Eq. (29a) and Eq. (29b) the explicit form of the stroboscopic map evolving the vector of expectation values is driven by two stochastic variables, one coming from the measurement and the other one from the imperfect feedback process. As discussed in the main text, we determine the optimal working value for the combined effect of these two stochastic quantities by minimizing $f_{\sigma_1,\sigma_2} = \sigma_1^2 + \sigma_2^2$. In order to derive a simple expression for the

optimal value of the measurement strength, we will assume $\Delta J_{z,i}^2 \approx \frac{J}{2}\sin(\theta_i)$, that is, the state remains almost a spin coherent state for all evolution times. As discussed above, this is a fair assumption within our protocol since the overall squeezing accumulated over time is small.

Similar to how we proceeded in Sec. I A we write $\sigma = \alpha\sqrt{J}$, and define a $f_{\sigma_1,\sigma_2}$ independent of the spin size

$$\tilde{f}_{\sigma_1,\sigma 2} = \frac{\alpha^2 + 1/2}{\alpha^4} + k^2\alpha^2 + \frac{k^2}{2}, \tag{31}$$

where $\tilde{f}_{\sigma_1,\sigma_2} = f_{\sigma_1,\sigma 2}J$. Looking for the extremal value one arrives at the condition

$$k^2\alpha^6 - \alpha^2\sin(\theta_i) - 1 = 0, \tag{32}$$

which can be reduced to a cubic algebraic equation by introducing $u = \alpha^2$. In Fig. 2 we show the some exemplary curves of the functions $\tilde{\Gamma}(\alpha)$ and $\tilde{f}_{\sigma_1,\sigma_2}(\alpha)$ as defined in Eq. (9) and Eq. (31), respectively. Notice how the location of the minimal value shifts to smaller $\alpha = \sigma/\sqrt{J}$ as we increase the value of $k$. However, this values is never too far from $\alpha \sim 0.9$.

### D. Calculation of $\Lambda_{\text{Largest}}$

The largest Lyapunov exponent provides information about a global properties of the chaotic phase. That is, it quantifies the average divergence (exponential) rate at which nearby initial conditions separate from each other in the chaotic sea. Locally, however, one can find different values for the exponent. We thus compute the largest Lyapunov exponent as the statistical average of local Lyapunov exponents associated with fiducial initial conditions all over phase space and define

$$\Lambda_{\text{Largest}} = \frac{1}{N_\Lambda}\sum_{j=1}^{N_\Lambda} \Lambda_{\text{Largest}}^{(\text{loc})}, \tag{33}$$

where $N_\Lambda$ is the number of fiducial initial conditions include in the average. The local Lyapunov exponent associated with each fiducial initial condition is calculated according to a standard procedure [? ]. We build an ensemble of nearby "shadow" initial conditions, evolve each of them and compute the distances between the fiducial trajectory to each of these trajectories. We average these distances over the ensemble of trajectories and extract the exponent from the slope of a linear fit to the portion of the mean separation distance that grows exponentially.

### E. Convergence of $\Lambda_{\text{Largest}}$ towards the classical value, the quantum to classical transition in the chaotic regime

We study the quantum-to-classical transition using quantum trajectories in the macroscopic limit [6]. We are particularly interested in the Lyapunov exponents associated with these trajectories. In doing so, a fundamental issue arises. We have noted that the stroboscopic map giving the evolution of the vector of expectation values is driven by two different stochastic variables. Though one can minimize, to some extent, the deleterious effects of these stochastic variables by working at an optimal measurement strength (see Fig. 2 (b)), the vector of expectation values evolves accordingly to a noisy dynamical system. The study of chaotic dynamics, as characterized by a positive Lyapunov exponent, in noisy systems is not a straightforward task [7]. In particular for Hamiltonian systems, where global chaos does not present a basis of attraction and in the long time limit distinguishing it from pure randomness is nearly impossible. Thus, calculation of Lyapunov exponents in our system for small values of $N$ is subtle.

Following [7] we calculate the divergence of nearby initial conditions, where the series of random numbers (the stochastic measurement record in our case) driving the evolution is different for each "shadow" trajectory. This method matches the classical exponents for a sufficient signal-to-noise ratio. In Fig. 3 we show the largest Lyapunov exponent as a function of the system size $N$, for (a) $k = 8$ and (b) $k = 10$. Notice how, as we decrease $N$ and do not satisfy the conditions under which quantum trajectories are a faithful representation of the classical dynamics [6], the and dynamics become dominated by measurement backaction noise. I this regime the value of exponent increases, as has been observe in other noisy dynamical systems [7]. This larger positive exponent is an artifact of the high level of noise and not chaos, since the real underlying dynamics rather than being nonlinear is simply a random walk, this case on the sphere. We observe the almost monotonically convergence of the exponent toward the appropriate classical value of the Lyapunov exponent (dashed black lines), and its respective standard deviation in the macrocopic limit.

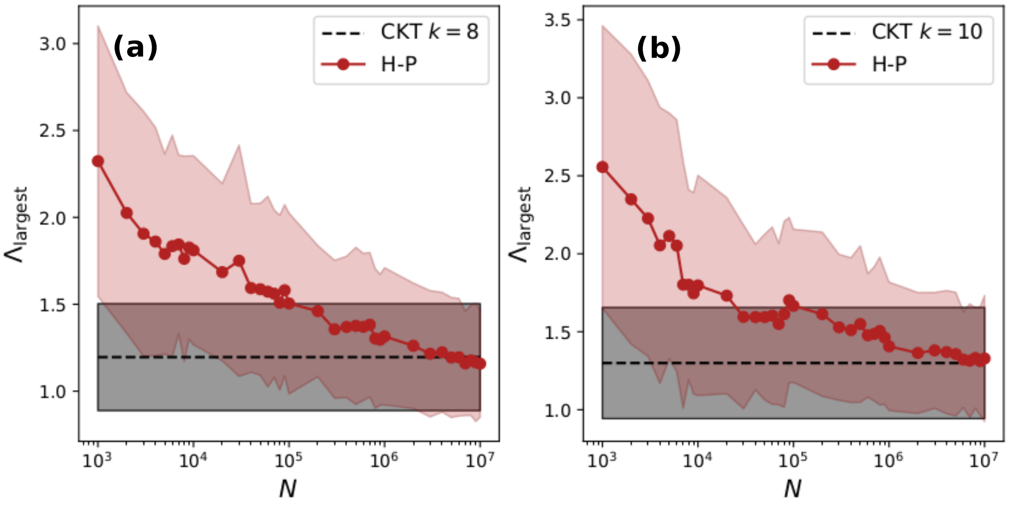


Figure 3. Largest Lyapunov exponent as a function of the system size for two different values of $k$ (red dots) and the corresponding value of the Lyapunov exponent for the classical map (dashed back line). **(a)** $k = 8$ and **(b)** $k = 10$.

## III. THE ATOM-LIGHT INTERFACE, OPTICAL PUMPING AND STOCHASTIC MASTER EQUATION

In this supplement we present the details of a model atom-light interface for QND measurement of the collective spin, and the concomitant decoherence that arises through the coupling to the meter. We consider an architecture consisting of an ensemble of ultracold atoms whose collective spin projection is continuously probed by an off-resonant laser beam through the Faraday interaction and polarization spectroscopy [8]. Photons scattered in to the forward direction of the beam ($z$-direction) are measured, while those diffusely scattered in $4\pi$ steradians are lost and are accompanied by optical pumping, leading to decoherence of the collective spin. Therefore a proper unraveling of the measurement model simulating the dynamics of the atom-light interface should capture the deleterious effects of optical pumping.

The description of this dynamics was introduced in [8]. We treat a simple 1D model, and ignore inhomogeneties in the atomic density and probe intensity as studied in detail in [9, 10]. Due to its interaction with the probe, and conditioned on the measurement record, the state of the collective spin evolves according to the stochastic master equation [9]

$$d\rho = \frac{\sqrt{\kappa}}{2}\mathcal{H}[\rho]dW + \frac{\kappa}{4}\mathcal{L}[\rho]dt + \gamma_s \sum_i \mathcal{D}_i[\rho]dt. \tag{34}$$

where $dW$ is a Wiener interval, $\gamma_s$ is the photon scattering rate for a unit oscillator strength, and $\kappa$ is the measurement rate. Here $\mathcal{H}[\rho]$ and $\mathcal{L}[\rho]$ are maps accounting for the random kicks and dephasing that arises as a consequences of the continuous monitoring of the collective spin. The last term accounts for optical pumping acting locally on the $i^{th}$ spin. These superoperators are given by

$$\mathcal{H}[\rho] = \{\rho, \hat{J}_z\} - 2\langle \hat{J}_z\rangle\rho, \tag{35a}$$

$$\mathcal{L}[\rho] = -\frac{1}{2}\{\rho, \hat{J}_z^2\} + \hat{J}_z\rho\hat{J}_z, \tag{35b}$$

$$\mathcal{D}_i[\rho] = -\{\rho, \hat{\Lambda}_i\} + \sum_q \hat{W}_{q,i}\rho\hat{W}_{q,i}^\dagger, \tag{35c}$$

where $\hat{\Lambda}_i$ represents absorption process and $\hat{W}_{q,i}$ are jump operators updating the state of the atom conditioned on the spontaneous emission of a photon with polarization $\boldsymbol{\epsilon}_q$ (the index $q$ runs over all elements of the spherical basis, see [8]).

We take a simple model of spin-1/2 ground state atoms and a laser tuned near a $S_{1/2} \to P_J$ transition (ignoring any nuclear spin and hyperfine splitting). The absorption and jump operators then take the form

$$\hat{\Lambda}_i = \frac{\mathbb{I}}{9}, \text{ and } \hat{W}_{q,i} = (\boldsymbol{\epsilon}_q^* \times \boldsymbol{\epsilon}_L) \cdot \frac{\hat{\boldsymbol{\sigma}}^{(i)}}{3}, \tag{36}$$

where $\boldsymbol{\epsilon}_L$ is the polarization vector of the light. Choosing, a linearly polarized probe in the $x$-direction, we can write

$$\hat{W}_{y,i} = -\frac{\hat{\sigma}_y^{(i)}}{3}, \text{ and } \hat{W}_{z,i} = \frac{\hat{\sigma}_x^{(i)}}{3}. \tag{37}$$

In usual experiments the quantization axis of the atoms is set by an external bias magnetic field in the direction of propagation of the light [11]. After going to the rotating frame with respect to this field and considering the operators in Eq. (36) and Eq. (37) the optical pumping map takes the form

$$\gamma_s \mathcal{D}_i[\rho] = -\gamma_{\rm OP}\rho + \frac{\gamma_{\rm OP}}{4}\hat{\sigma}_x^{(i)}\rho\hat{\sigma}_x^{(i)} + \frac{\gamma_{\rm OP}}{4}\hat{\sigma}_y^{(i)}\rho\hat{\sigma}_y^{(i)} + \frac{\gamma_{\rm OP}}{2}\hat{\sigma}_z^{(i)}\rho\hat{\sigma}_z^{(i)}, \tag{38}$$

where $\gamma_{\rm OP} = \frac{2}{9}\gamma_s$ is the optical pumping rate for flipping the spin.

For the large ensembles under consideration here, e.g. $N \sim 10^6$, we work under the Gaussian approximation, where third-order moments of commuting observables can be expressed using first- and second-order moments under the relation $\langle \hat{X}\hat{Y}\hat{Z}\rangle = \langle \hat{X}\hat{Y}\rangle\langle \hat{Z}\rangle + \langle \hat{X}\hat{Z}\rangle\langle \hat{Y}\rangle + \langle \hat{Y}\hat{Z}\rangle\langle \hat{X}\rangle - 2\langle \hat{X}\rangle\langle \hat{Y}\rangle\langle \hat{Z}\rangle$ [3]. We write equations of motion for the vector of mean values and the entries of the covariance matrix $d\langle \hat{J}_i\rangle = \mathrm{Tr}\left(\hat{J}_i d\rho\right)$, $d\langle \Delta\hat{J}_i^2\rangle = \mathrm{Tr}\left(\Delta\hat{J}_i^2 d\rho\right)$, $d\mathbb{V}_{i,j} = \mathrm{Tr}\left(\mathbb{V}_{i,j} d\rho\right)$. When computing the traces in these expressions it is convenient to have idea of how one- and two- body correlations evolve under the action of the optical pumping map in Eq. (38). It can be shown that these correlations evolve as

$$\left.\frac{d\langle \hat{o}^{(i)}\rangle}{dt}\right|_{\rm OP} = \langle \gamma_s\mathcal{D}_i[\hat{o}^{(i)}]\rangle, \text{ and } \left.\frac{d\langle \hat{o}^{(i)}\hat{a}^{(i)}\rangle}{dt}\right|_{\rm OP} = \langle \gamma_s\mathcal{D}_i[\hat{o}^{(i)}]\hat{a}^{(i)}\rangle + \langle \hat{o}^{(i)}\gamma_s\mathcal{D}_i[\hat{a}^{(i)}]\rangle, \tag{39}$$

where $\hat{o}^{(i)}$ and $\hat{a}^{(i)}$ are operators acting on individual spins in the ensemble.

Using these relations we write the set of coupled stochastic differential equations evolving the vector of mean values and the entries of the covariance matrix as

$$d\langle \hat{J}_x\rangle = -\left(\frac{\kappa}{8} + 3\gamma_{\rm OP}\right)\langle \hat{J}_x\rangle dt + \sqrt{\kappa}\mathbb{V}_{z,x}dW, \tag{40a}$$

$$d\langle \hat{J}_y\rangle = -\left(\frac{\kappa}{8} + 3\gamma_{\rm OP}\right)\langle \hat{J}_y\rangle dt + \sqrt{\kappa}\mathbb{V}_{z,y}dW, \tag{40b}$$

$$d\langle \hat{J}_z\rangle = -2\gamma_{\rm OP}\langle \hat{J}_z\rangle dt + \sqrt{\kappa}\langle \Delta\hat{J}_z^2\rangle dW, \tag{40c}$$

$$d\langle \Delta\hat{J}_x^2\rangle = \left(\frac{\kappa}{4}\langle \hat{J}_y\rangle^2 + \frac{\kappa}{4}\langle \Delta\hat{J}_y^2\rangle - \frac{\kappa}{4}\langle \Delta\hat{J}_x^2\rangle - \kappa\mathbb{V}_{x,z}^2 - 3\gamma_{\rm OP}\langle \Delta\hat{J}_x^2\rangle + 3N\frac{\gamma_{\rm OP}}{4}\right)dt, \tag{40d}$$

$$d\langle \Delta\hat{J}_y^2\rangle = \left(\frac{\kappa}{4}\langle \hat{J}_x\rangle^2 + \frac{\kappa}{4}\langle \Delta\hat{J}_x^2\rangle - \frac{\kappa}{4}\langle \Delta\hat{J}_y^2\rangle - \kappa\mathbb{V}_{y,z}^2 - 3\gamma_{\rm OP}\langle \Delta\hat{J}_y^2\rangle + 3N\frac{\rm OP}{4}\right)dt, \tag{40e}$$

$$d\langle \Delta\hat{J}_z^2\rangle = \left(-\kappa\langle \Delta\hat{J}_z^2\rangle^2 - 2\gamma_{\rm OP}\langle \Delta\hat{J}_z^2\rangle + N\frac{\gamma_{OP}}{2}\right)dt, \tag{40f}$$

$$d\mathbb{V}_{z,x} = \left(-\frac{\kappa}{8}\mathbb{V}_{x,z} - \kappa\langle \Delta\hat{J}_z^2\rangle\mathbb{V}_{x,z} + \frac{5}{2}\gamma_{\rm OP}\mathbb{V}_{x,z}\right)dt, \tag{40g}$$

$$d\mathbb{V}_{z,y} = \left(-\frac{\kappa}{8}\mathbb{V}_{y,z} - \kappa\langle \Delta\hat{J}_z^2\rangle\mathbb{V}_{y,z} + \frac{5}{2}\gamma_{\rm OP}\mathbb{V}_{y,z}\right)dt, \tag{40h}$$

$$d\mathbb{V}_{x,y} = \left(-\frac{\kappa}{2}\mathbb{V}_{x,y} - \frac{\kappa}{4}\langle \hat{J}_x\rangle\langle \hat{J}_y\rangle - \kappa\mathbb{V}_{x,z}\mathbb{V}_{y,z} - 3\gamma_{\rm OP}\mathbb{V}_{x,y}\right)dt. \tag{40i}$$

This set of equations in conjunction with $\mathcal{M}(t)dt = \langle \hat{J}_z\rangle dt + \frac{1}{\sqrt{\kappa}}dW$ to simulate the measurement record, implement the measurement part of our map. The numerical integration of these coupled stochastic differential equations is done with an improved Euler scheme [12].

Using these stochastic equations, we can calculate how decoherence limits our ability to perform a QND measurement, which is at the heart of our measurement-based feedback protocol. Fundamentally, the measurement is performed by detecting the photons that are forward-scattered into the probe, but information about the spins is also lost in the diffuse scattering of photons in $4\pi$ steradians, which limits the measurement strength we can achieve. As presented in Fig. 4d of the main text, we can reliably extract Lyapunov exponents for an optical density of 300, the parameter that quantifies the ratio of cooperative forward scattering to diffuse scattering. This means that the required exponential growth of the separation between nearby trajectories can be seen within the time scale set by the decoherence for the above given value of cooperativity. Currently, many experiments based on a free space atom-light interface achieve smaller values of OD. To address this, in in Fig. 4a we present the calculation of the largest Lyapunov

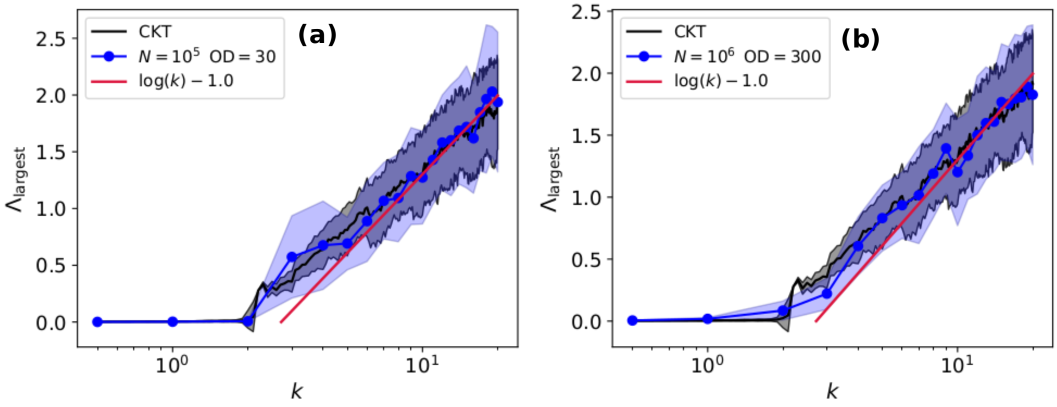


Figure 4. Largest Lyapunov exponent as a function of the chaoticity parameter $k$ computed with the method presented in Sec. II D (blue dots), for comparison we include the exponent as calculated for the CKT (black continuous) and an analytical expression known to approximate the value at large $k$ (continuous red). The difference between left and right steams in the value of the optical density with, **(a)** OD = 30, $N = 10^5$, and **(b)** OD = 300, $N = 10^6$.

exponent for OD = 30. For this smaller cooperativity, we see some variations with respect to the case of OD = 300 (Fig. 4)b and the ideal case (Fig. (4)c of main text). Nonetheless, even for such relatively large rates of decoherence relative to the measurement rate, we see an overall good agreement with the classical exponent. Thus, even when we are forced to work within a shorter time span before the signal decays, the exponential growth of the separation distance can still be observed.


[1] J. Audretsch, L. Diósi, and T. Konrad, Physical Review A **66**, 022310 (2002).
[2] T. Holstein and H. Primakoff, Physical Review **58**, 1098 (1940).
[3] K. Jacobs and D. A. Steck, Contemporary Physics **47**, 279 (2006).
[4] A. Kuzmich, L. Mandel, and N. P. Bigelow, Physical Review Letters **85**, 1594 (2000).
[5] J. K. Stockton, R. van Handel, and H. Mabuchi, Physical Review A **70**, 022106 (2004).
[6] T. Bhattacharya, S. Habib, and K. Jacobs, Physical Review Letters **85**, 4852 (2000).
[7] G. Boffetta, M. Cencini, M. Falcioni, and A. Vulpiani, Physics Reports **356**, 367 (2002).
[8] I. H. Deutsch and P. S. Jessen, Optics Communications **283**, 681 (2010).
[9] B. Q. Baragiola, L. M. Norris, E. Montaño, P. G. Mickelson, P. S. Jessen, and I. H. Deutsch, Physical Review A **89**, 033850 (2014).
[10] L. M. Norris, *Internal Spin Control, Squeezing and Decoherence in Ensembles of Alkali Atomic Spins*, Ph.D. thesis (2014), arXiv:1410.0089.
[11] E. Montano, D. Hemmer, B. Q. Baragiola, L. M. Norris, E. Shojaee, I. H. Deutsch, and P. S. Jessen, (2018), arXiv:1811.02519.
[12] A. J. Roberts, (2012), arXiv:1210.0933.
